# Supplementary material for: Designing angle-independent structural colors using Monte Carlo simulations of multiple scattering
Source: arXiv:2007.14831 ancillary file (2020-07-29)
Supplement: Supplementary file 1 [file SI_appendix.pdf]

# Supplementary Information for

## Prediction and design of angle-independent structural colors from Monte Carlo simulations of multiple scattering

**Victoria Hwang, Anna B. Stephenson, Solomon Barkley, Soeren Brandt, Ming Xiao, Joanna Aizenberg, and Vinothan N. Manoharan**

**Vinothan N. Manoharan.**
**E-mail: vnm@seas.harvard.edu**

### This PDF file includes:

Supplementary text
Figs. S1 to S3
SI References

## Supporting Information Text

## Materials and Methods

**Fabrication of samples.** To validate our model, we make angle-independent structurally colored films with varying nanoparticle size, volume fraction, thickness, number of components, and carbon black concentration. In most samples, we use polystyrene nanoparticles of sizes ranging from 190 nm to 280 nm in diameter, and mixtures of two different diameters for the binary films. The protocol used to synthesize the particles can be found in Refs. 1 and 2. The nanoparticles are suspended in salt water at 25 mM NaCl (50 mM for the 280 nm particle). The salt screens the electrostatic interactions between the particles and prevents the films from crystallizing. We centrifuge the suspensions for 40 min to 60 min at 14000$g$. We remove the supernatant and vortex and sonicate for 10 min to resuspend the particles. The final concentration of the particles is between 35 and 45% v/v. To make films with carbon black, we add different volumes of 1% w/w carbon black suspension to the particle suspensions, keeping their final concentrations between 38 and 42% v/v.

We make films that are thicker than 20 µm by injecting the concentrated suspensions into a sample chamber, which we make by sandwiching Mylar spacers of varying thicknesses between glass slides and glass coverslips and sealing with UV-curable epoxy. To make films of polystyrene particles in air, we inject suspensions at 45% v/v into sample chambers and leave a pool of excess suspension at the inlet. We periodically refill this pool over 6 h to 8 h as the water evaporates from the outlet, densely packing the particles and pulling in more suspension through capillary action. We dry the samples overnight at room temperature and remove any excess water by drying them in an oven at 60 °C for several hours.

To make films that are thinner than 20 µm, we spin coat (Laurell WS-650Mz-23NPP) a dense suspension of particles in 50 mM NaCl onto a glass slide at 1000 rpm and 2000 rpm for 2 min with an acceleration of 500 rpm/s. We use more salt than in the thicker samples because the forces during spin coating can align the particles into crystalline domains. We let the thin films air dry overnight before measuring their reflectance.

Finally, we make a thick 3930 µm-film using a drop-casting method, in which we fill a cylindrical tube of 7 mm in diameter and 1 cm in height with a 45% v/v particle suspension and let it dry overnight. The tube, the ends of which are open on both sides, is placed on a gypsum substrate that absorbs water quickly, allowing for rapid drying and assembling of the particles into a thick amorphous film.

**Measurement of reflectance spectra.** We measure the reflectance spectra of structurally colored films with a spectrophotometer containing an integrating sphere (Agilent Cary 7000 Universal Measurement Spectrophotometer) that collects all the light scattered into the reflection hemisphere. We normalize the measurement with a white diffuse reflectance standard (Spectralon, Labsphere). The sample is illuminated with light from a double out-of-plane Littrow monochromator on a 1 mm × 3 mm rectangular spot. The port where the sample is placed is a circular opening 6 mm in diameter. We calculate error bars (shown in gray in spectral data) as two standard deviations about the mean of measurements taken at 4 to 11 different locations on the samples, unless otherwise noted in the text.

We use the same procedure to measure the reflectance of the mountain bluebird specimen (Specimen MCZ:Orn:190556. *Sialia currucoides.* North America: United States: Montana: Meagher. Martinsdale. Robert S. Willians; Ornithology Department of the Museum of Comparative Zoology at Harvard University). We measure the blue region on the back of the bird. We measure three spots on the same region to account for inhomogeneities in the color, and we convert the average reflectance spectra into a color swatch using the software package ColorPy (3). We use the CIELAB coordinates of the swatch as a target color.

**Measurement of sample parameters.** To validate our model, we measure the experimental properties of our films that are required by the model: particle radius and polydispersity, volume fraction, film thickness, and particle and matrix complex refractive indices.

To determine the volume fraction of our films of polystyrene particles in water, we calculate the

concentration of particles after centrifuging and removing controlled amounts of supernatant water. We measure the initial concentration of the suspension by gravimetric analysis. To estimate the volume fraction of our films of polystyrene in air, we divide the weight of the packing by the density of the particles to get the volume of the particles in the chamber. We divide this volume by the total volume of the chamber to get the final volume fraction.

We measure the mean particle diameter from dozens of measurements from scanning electron microscopy images (Ultra Plus Field Emission Scanning Electron Microscope). The polydispersity is given by the root-mean-square deviation in the measured values divided by the mean particle diameter.

We measure the thickness of our films by measuring with a micrometer the total thickness of the sample chamber and subtracting the thickness of the glass substrate and the coverslip cover. We perform this measurement on roughly ten areas of the sample and use the mean value for our calculations. For the 3930 µm-film, we measure the thickness directly with a micrometer, and for the thin 7 µm and 18 µm-films, we measure the thickness from scanning electron microscopy images (scanning electron microscope JEOL JSM-6390LV)

We estimate the real part of the refractive index of the polystyrene particles using the Sellmeier dispersion formula with parameters that were fit to experimental data (4). Polystyrene particles are not completely lossless (5). To estimate the imaginary component of the refractive index of the polystyrene particles, we index-match the polystyrene with a Cargille oil (series E n(5893 Å) 25° C = 1.5800). We then measure the extinction of the suspension using a spectrophotometer (NanoDrop 1000, Thermo Fischer Scientific) and we use the Cargille oil as a reference liquid. We assume that the extinction comes only from the absorption in the polystyrene particles because the scattering is suppressed, owing to the index match. We ignore the absorption in the Cargille oil because it is 1 to 2 orders of magnitude smaller than the absorption in the polystyrene particles. Then the imaginary component of the refractive index $n_i$ of polystyrene is

$$n_i = \frac{\mu_{\text{abs}}\,\lambda}{4\pi}, \tag{1}$$

where $\lambda$ is the wavelength in vacuum and $\mu_{\text{abs}}$ is the absorption coefficient of one particle:

$$\mu_{\text{abs}} = \frac{\mu_{\text{abs,system}}}{v_f} \tag{2}$$

$$\mu_{\text{abs,system}} = \frac{A}{l}, \tag{3}$$

where $\mu_{\text{abs,system}}$ is the absorption coefficient of the system of particles, $v_f$ is the volume fraction of the particles in the oil, $A$ is the absorbance, and $l$ is the path length in the spectrophotometer measurement. We measure the imaginary refractive index of the different polystyrene particles we use. The 188 nm particles have an average imaginary index between $2 \times 10^{-5}i$ and $2 \times 10^{-4}i$, and we choose a constant value of $2 \times 10^{-5}i$ in our calculations. The 202 nm particles have an average imaginary index between $3.5 \times 10^{-5}i$ and $6.5 \times 10^{-5}i$, and we choose a constant value of $6 \times 10^{-5}i$ in our calculations. The 218 nm particles have an imaginary index between $2.5 \times 10^{-5}i$ and $1.9 \times 10^{-3}i$, and we use a constant value of $3 \times 10^{-5}i$. The 276 nm particles have an imaginary index between $1.6 \times 10^{-5}i$ and $5.7 \times 10^{-5}i$, and we use a constant value of $2 \times 10^{-5}i$.

In the samples with carbon black, we convert the carbon black concentration to the imaginary index of the sample by substituting Eq. (2) for a carbon black nanoparticle into Eq. (1):

$$n_i = v_f\, n_{i,\text{CB}}, \tag{4}$$

where now $v_f$ is the volume fraction of carbon black in the sample and $n_{i,\text{CB}}$ is the imaginary refractive index of carbon black. In our calculations we use $n_{i,\text{CB}} = 0.44\,i$, which is commonly used in the literature (6–8). To estimate the volume fraction of carbon black in the samples, we assume a carbon black density of $2\,\text{g/cm}^3$. We solve for the matrix imaginary index from the sample imaginary index $n_i$ using Bruggeman's

formula. We input this matrix imaginary index into our calculations to validate the model with samples with carbon black.

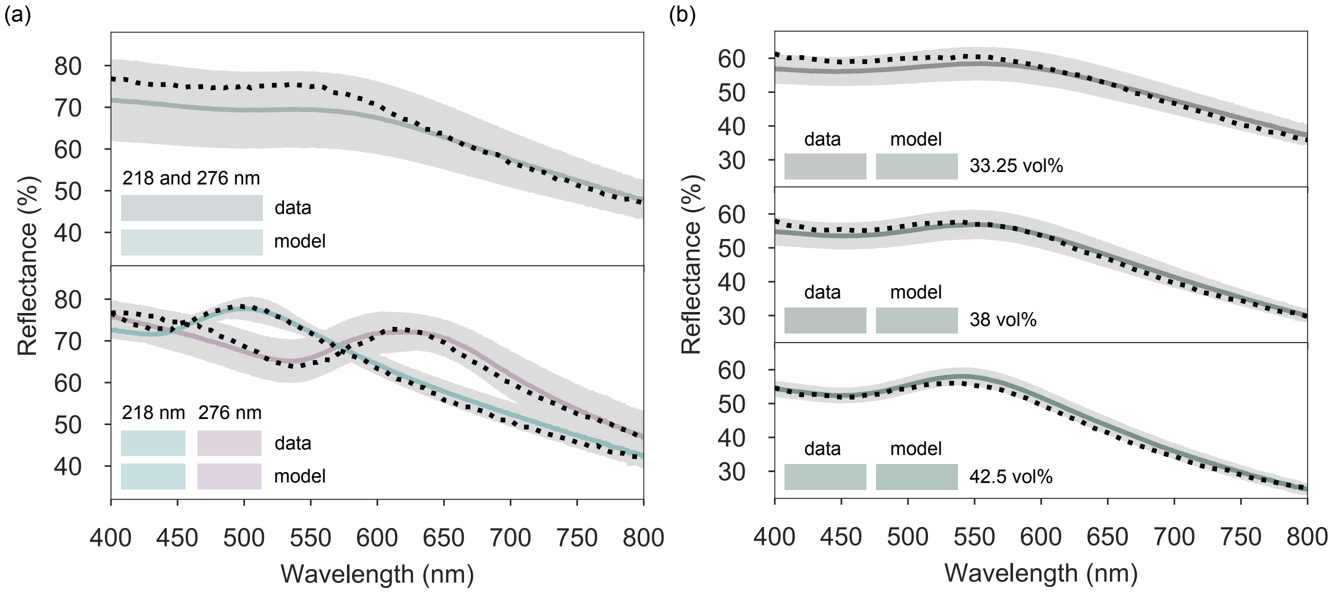


**Fig. S1.** Additional validations of the Monte Carlo model. Experimental reflectance spectra for films of polystyrene are shown by the solid lines and predicted spectra by the dotted lines. Error bars are shown in gray. The colors of the insets correspond to the ColorPy swatches generated from the experimental and predicted spectra. The sample parameters are as follows: (a) (top) Binary mixture of 218 nm and 276 nm diameter particles (2:1 by number) in air. The volume fraction is 0.52, the thickness is 85 µm, the fine roughness is 0.5, and the coarse roughness is 0.9. Error bars are two standard deviations from nine measurements on different locations on the sample. (a) (bottom) Same 218 nm and 276 nm particle samples as Fig. 3a in main text shown for comparison against the binary mixture. (b) Diameter of 202 nm polystyrene particles in water at volume fractions of 0.3325, 0.38, and 0.425. The corresponding thicknesses are 84 µm, 79 µm and 90 µm. The fine roughness is 0.28, and the coarse roughness is 0.2. Error bars are two standard deviations from six, fifteen, and nine measurements on different locations on the samples.

Lastly, we specify the incident illumination angles and detection angles in the calculations. The incident illumination angle is the angle between the light source and the normal to the film, and we use a value of 8° based on the integrating sphere geometry. The detection angle is the range of angles captured by the detector—when the detection angle is 0°, only the backscattered light is detected, and when the angle is 90°, the entire reflection hemisphere is captured. In most of our calculations, we use a value of 90° since the integrating sphere should capture all the reflected light. However, we measure some samples on the side of the chamber that contains epoxy glue, which adds a small gap between the film and the aperture, decreasing the detection angle. These samples are the blue and pink films in Fig. 3a, for which we use detection angles of 80°, and the binary sample in Fig. S1a, for which we use a detection angle of 75°.

## Model details

**Monte Carlo trajectories.** In the model, the photon packets have initial positions, directions, and weights. The positions are the ($x$, $y$, $z$)-coordinates in the sample's reference frame, and the packets start at $z = 0$ and are randomly distributed along $x$ and $y$. The directions are the directions of propagation after each scattering event and are initially in $+z$ if the sample surface is smooth. The weights account for absorption in the sample, which comes from a non-zero imaginary refractive index of any of the sample materials. As photon packets travel through the sample, they are absorbed according to the Beer-Lambert law and their weights decrease accordingly. The initial normalized weights for all packets is 1.

The model samples the step sizes and the directions of propagation after each scattering event from two distributions. The step size distribution is based on Beer's law:

$$p(\text{step}) = \frac{1}{l_{\text{sca}}} e^{-\frac{\text{step}}{l_{\text{sca}}}}, \tag{5}$$

 

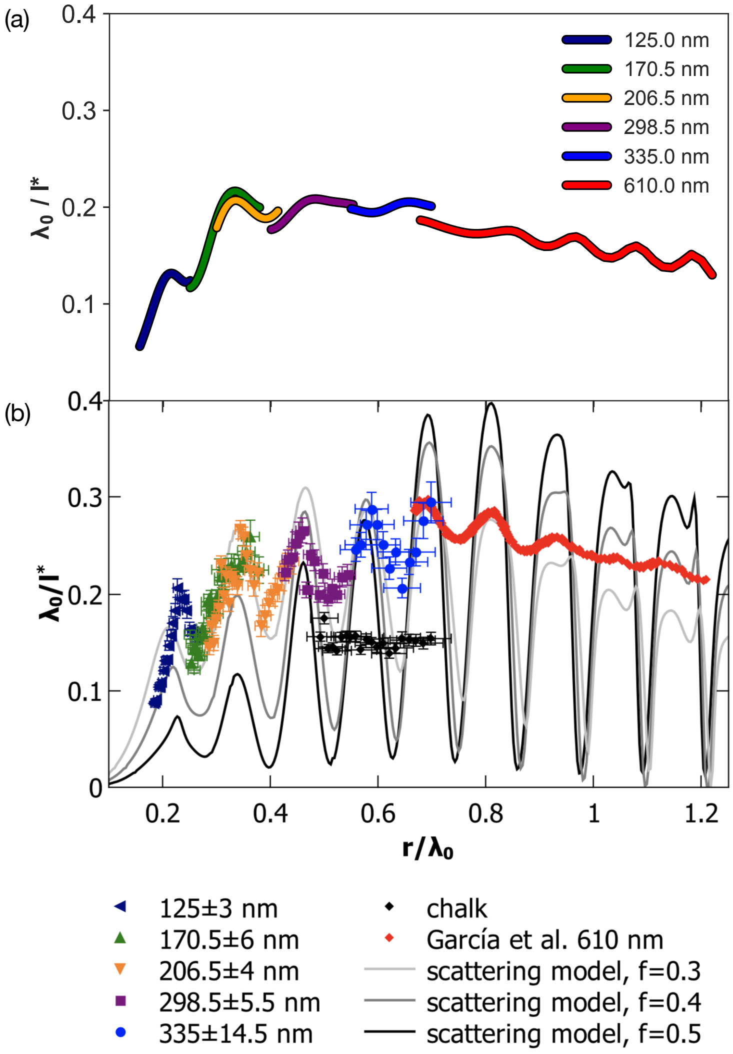


**Fig. S2.** (a) Scattering strength of polystyrene particles with radius 125 nm to 610 nm calculated with the Bruggeman effective approximation at a volume fraction of 0.3. (b) Scattering strength of polystyrene particles calculated with the energy coherent potential approximation (ECPA). Reprinted Figure 4 with permission from Ref. 9 as follows: Geoffroy J. Aubry, Lukas Schertel, Mengdi Chen, Henrik Weyer Christof M. Aegerter, Sebastian Polarz, Helmut Coelfen, and Georg Maret, *Phys. Rev. A* **96**, 043871, 2017 (`http://dx.doi.org/10.1103/PhysRevA.96.043871`). Copyright 2017 by the American Physical Society. Colored data points correspond to measured values, and gray lines correspond to the predictions using ECPA at different volume fractions. (a) and (b) share the same $x$-axis.

and its mean is the scattering length:

$$l_{\text{sca}} = \frac{1}{\rho\, C_{\text{sca}}^{\text{sample}}}. \tag{6}$$

Here $p(\text{step})$ is the probability of a step size, $\rho$ is the number density of scatterers, and $C_{\text{sca}}^{\text{sample}}$ is the scattering cross-section of the sample calculated with an adapted version of the single-scattering model (10) that uses Bruggeman's approximation (11) for the effective refractive index of the sample. The distribution for the direction of propagation is the phase function, which describes the probability that light will be scattered in a certain direction:

$$p(\theta) = \frac{\mathrm{d}C_{\text{sca}}^{\text{sample}}}{\mathrm{d}\Omega}\,\frac{1}{C_{\text{sca}}^{\text{sample}}}, \tag{7}$$

where $p(\theta)$ is the phase function at scattering angle $\theta$ and $\mathrm{d}C_{\text{sca}}^{\text{sample}}/\mathrm{d}\Omega$ is the differential scattering cross-section of the sample calculated with the single-scattering model.

The Bruggeman approximation for the effective index of the sample is

$$\begin{gathered}\sum_{j=1}^{N} f_j\,\frac{n_j^2 - n_{\text{BG}}^2}{n_j^2 + 2\,n_{\text{BG}}^2} = 0\\ \sum_{j=1}^{N} f_j = 1,\end{gathered} \tag{8}$$

where $N$ is the number of components in the sample, $f_j$ is the volume fraction of component $j$ and $n_j$ its complex index, and $n_{\text{BG}}$ is the complex Bruggeman effective index of the sample. We choose Bruggeman's formula as opposed to the commonly used Maxwell-Garnett approximation because Bruggeman is a symmetric formula and should therefore be more appropriate at volume fractions near 0.5 (11), as found in our experimental samples.

***Implementation of absorption.*** The absorption of light by a material is determined by the imaginary component of its refractive index. Therefore, to incorporate the effect of absorption, we use complex refractive indices for the particle and the matrix in the calculation of the effective index. The resulting complex index leads to complex values for the size parameter $x$, index ratio $m$, and wavevector $k$. To correctly account for these quantities in Mie theory, we use a form of the Mie scattering coefficients $a_n$ and $b_n$ that is computationally stable (12, 13) for complex values:

$$a_n = \frac{[D_n(mx)/m + n/x]\,\psi_n(x) - \psi_{n-1}(x)}{[D_n(mx)/m + n/x]\,\xi_n(x) - \xi_{n-1}(x)} \tag{9}$$

$$b_n = \frac{[mD_n(mx) + n/x]\,\psi_n(x) - \psi_{n-1}(x)}{[mD_n(mx) + n/x]\,\xi_n(x) - \xi_{n-1}(x)}, \tag{10}$$

where $D_n$ is the logarithmic derivative defined as

$$D_n(\rho) = \frac{d}{d\rho}\ln\psi_n(\rho), \tag{11}$$

and $\psi_n$ and $\xi_n$ are the Riccati-Bessel functions that depend on the spherical Bessel functions $j_n$ and $y_n$:

$$\psi_n(\rho) = \rho j_n(\rho) \tag{12}$$
$$\xi_n(\rho) = \rho\,[j_n(\rho) + iy_n(\rho)]. \tag{13}$$

We compute the spherical Bessel functions with the functions `spherical_jn()` and `spherical_yn()` from the package `scipy`.

We must also avoid the far-field approximation to the Mie solutions commonly used in non-absorbing systems. In this approximation, the differential scattering cross-section of the particle is integrated in the far field, where the computation is simplified. But in an absorbing sample, the cross section decreases with distance, and the integration in the far field gives unphysical results. We could instead use the generalized Mie solutions to calculate the differential cross-section and integrate it at the surface of the particle, but the generalized Mie solutions include near fields. Given that the near fields decay over distances much shorter than the scattering length, we can ignore the near fields while integrating the differential scattering cross-section at the surface of the particle (Figure 2c). We do this by using the far-field solutions for the scattered fields (12):

$$E_{s\theta} \sim E_0 \frac{e^{ikr}}{-ikr} \cos\phi \, S_2(\cos\theta) \tag{14}$$

$$E_{s\phi} \sim E_0 \frac{e^{ikr}}{-ikr} \sin\phi \, S_1(\cos\theta), \tag{15}$$

where $S_1$ and $S_2$ are the diagonal elements of the amplitude scattering matrix, $\theta$ is the scattering angle, $\phi$ is the azimuthal angle, $E_0$ is the incident field, and $r$ is the distance from the center of the particle. We calculate the differential scattering cross-section by multiplying the scattered fields by their complex conjugates. Because $k$ is complex, the exponential factor in Eq. (14) and Eq. (15) becomes $e^{-2k''r}$, and the remaining $r$-dependence becomes $1/[(k'r)^2+(k''r)^2]$, where $k'$ and $k''$ are the real and imaginary components of $k$ (14). If the system is non-absorbing, these factors reduce to $1/(kr)^2$, and the $1/r^2$-dependence cancels in the integration of the differential scattering cross-section in spherical coordinates. If the system is absorbing, we perform the integration at $r = a$, where $a$ is the radius of the particle. To account for the decay in intensity between scattering events, we decrease the weight of the trajectories based on the distance traveled in the sample according to the Beer-Lambert law. Finally, we include a correction factor that accounts for the variation in the amplitude of the incident intensity $I_0$ at different locations of the particle (15):

$$I_{0,\text{corrected}} = 2I_0 \left[ \frac{e^{2ak''}}{2ak''} + \frac{1 - e^{2ak''}}{(2ak'')^2} \right]. \tag{16}$$

***Implementation of polydisperse and multilayered particles.*** To model systems with polydisperse particles or with two mean diameters, we compute the scattered intensity $I$ using polydisperse form and structure factors (16):

$$I \propto \overline{F(q)} * S_M(q) \tag{17}$$

where $\overline{F(q)}$ is the polydisperse form factor derived from a size average (1) and $S_M(q)$ is the polydisperse measurable structure factor (17). This structure factor assumes a Schulz distribution for the particle diameter, which tends to a Gaussian distribution when the polydispersity is small.

We also model systems of multilayered particles where the core and the shells are made of different materials. We calculate the scattering coefficients of multilayered particles following the approach in Ref. 18. In addition to replacing the Riccati-Bessel functions with their logarithmic derivatives (Eq. (11)), we calculate the internal and external fields as a superposition of inward and outward waves with radial dependences described by the spherical Bessel and Hankel functions of the first kind. We also use an up-recursion algorithm to calculate a ratio of the Riccati-Bessel functions that is numerically stable at large size parameters. The scattering coefficients calculated through this approach are used to compute the form factor in the model. To calculate the structure factor, we use the size parameter corresponding to the largest radius of the multilayered particle.

To calculate the effective index of the sample when the particles are multilayered, we take advantage of the fact that the Bruggeman formula can be used for an arbitrary number of components. We calculate the volume fraction of each layer in the sample and solve for the effective Bruggeman index in Eq. (8). This approach must be used with caution because Eq. (8) assumes that each component is surrounded by the effective index set by the component and the matrix. However, this approach was also implemented in a

single-scattering model and was shown to reasonably predict the features of reflectance spectra of hollow carbon-silica core-shell particles (19).

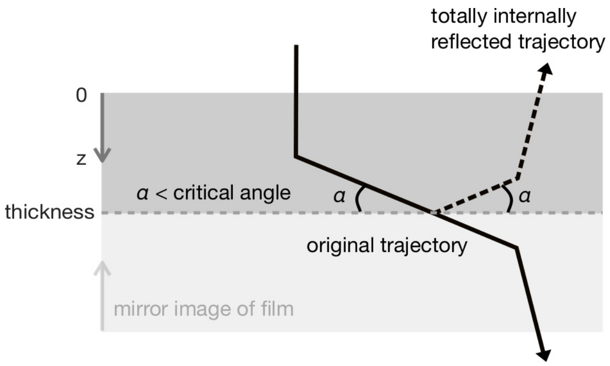


**Fig. S3.** Illustration of how the Monte Carlo model accounts for totally internally reflected trajectories.

***Implementation of boundary effects.*** The film has interfaces at the top and bottom boundaries that cause reflection and refraction of light. We use the Fresnel equations to calculate the fraction of trajectories that are reflected at the top interface when light goes from the medium index to the sample effective index, and similarly when light exits through the bottom boundary from the sample effective index to the medium. Because films are sometimes prepared in sample chambers, we can specify the refractive index of a homogeneous material, such as glass, that lies between the top and bottom interfaces of the film and the medium. In addition, light refracts as it enters and exits the sample, and we use Snell's law to calculate the initial and final directions of the trajectories.

When a trajectory hits a boundary at an angle that is smaller than the critical angle, it must be counted as totally internally reflected instead of refracted by the interface. To optimize running time and avoid generating a new totally trajectory, we assume that the original trajectory is located in a mirror image of the film. Then, if the original trajectory exits the mirror image through the bottom interface, we count it as a totally internally reflected trajectory that exits the top boundary of the original film (Fig. S3). This mirror-image approach can be used for multiple total internal reflections.

***Effect of surface scattering.*** To use the multiple-scattering model as a quantitative tool for color prediction, we incorporate the effect of surface scattering in our calculations. We model the surface roughness as coarse or fine, depending on whether the roughness is large or small relative to the wavelength of light. The coarse roughness parameter is defined as the root-mean-square of the slope of the surface (20), and the effect of this parameter on our calculations is that it modifies the angles of refraction and Fresnel reflection when light hits the interface. Therefore, the first step of the trajectories is taken in a direction that is not necessarily in $+z$. While the coarse roughness is theoretically measurable, experimental characterization is unfeasible for many of our samples where standard profilometry techniques cannot be used (such as in our samples of polystyrene particles in water). Therefore, we fit the value of coarse roughness but we keep it constant for the same sample assembly technique, since we expect the shape of the sample interface to depend largely on the drying phenomena and packing processes that occur while making our samples.

While the coarse roughness improves the agreement between model and data, it still assumes an interface where light travels from the medium refractive index to the sample effective index, and thus still suffers from the invalidity of effective-medium theory at the boundary of a sample. The fine roughness corrects for this invalidity by assuming that light does not necessarily encounter an interface described by an effective medium, but is rather scattered by individual particles or clusters of particles that protrude from the boundary. When light encounters fine roughness, we keep all our calculations the same except for the first step size, which is computed without the contribution of the structure factor, meaning that we only use Mie theory to calculate the scattering length distribution from which we sample the first step size.

All the following steps are sampled normally: from a distribution whose mean is the scattering length calculated with both the form and structure factors. We therefore define the fine roughness as the fraction of trajectories whose first step is sampled from a distribution that excludes the structure factor. When we include both fine and coarse roughness parameters, we add both effects—we sample the first step size from a distribution based on Mie theory and find new angles of refraction and reflection of the incident trajectories to account for the surface tilt.

## References


1. Hwang V, Stephenson AB, Magkiriadou S, Park JG, Manoharan VN (2020) Effects of multiple scattering on angle-independent structural color in disordered colloidal materials. *Physical Review E* 101(1):012614.
2. Park JG, et al. (2017) Photonic-crystal hydrogels with a rapidly tunable stop band and high reflectivity across the visible. *Optical Materials Express* 7(1):253–263.
3. Kness M (2008) ColorPy - A python package for handling physical descriptions of color and light spectra. The source package can be found at https://github.com/markkness/ColorPy.
4. Sultanova N, Kasarova S, Nikolov I (2009) Dispersion Properties of Optical Polymers. *Acta Physica Polonica A* 116(4):585–587.
5. Ma X, et al. (2003) Determination of complex refractive index of polystyrene microspheres from 370 to 1610 nm. *Physics in Medicine and Biology* 48(24):4165–4172.
6. Chýlek P, Videen G, Ngo D, Pinnick RG, Klett JD (1995) Effect of black carbon on the optical properties and climate forcing of sulfate aerosols. *Journal of Geophysical Research* 100(D8):16325.
7. D'Almeida GA, Koepke P, Shettle EP (1991) *Atmospheric aerosols: global climatology and radiative characteristics*, Studies in geophysical optics and remote sensing. (A. Deepak Pub, Hampton, Va., USA).
8. Kou L (1996) Ph.D. thesis.
9. Aubry GJ, et al. (2017) Resonant transport and near-field effects in photonic glasses. *Physical Review A* 96(4):043871.
10. Magkiriadou S, Park JG, Kim YS, Manoharan VN (2014) Absence of red structural color in photonic glasses, bird feathers, and certain beetles. *Physical Review E* 90(6):062302.
11. Markel VA (2016) Introduction to the Maxwell Garnett approximation: tutorial. *Journal of the Optical Society of America A* 33(7):1244.
12. Bohren CF, Huffman DR (2004) *Absorption and scattering of light by small particles.* (Wiley-VCH Verlag GmbH Co. KGaA).
13. Frisvad JR, Christensen NJ, Jensen HW (2007) Computing the scattering properties of participating media using Lorenz-Mie theory. *ACM Transactions on Graphics* 26(3):60.
14. Mundy WC, Roux JA, Smith AM (1974) Mie scattering by spheres in an absorbing medium. *Journal of the Optical Society of America* 64(12):1593.
15. Sudiarta IW, Chýlek P (2001) Mie-scattering formalism for spherical particles embedded in an absorbing medium. *Journal of the Optical Society of America A* 18(6):1275.
16. Scheffold F, Mason TG (2009) Scattering from highly packed disordered colloids. *Journal of Physics: Condensed Matter* 21(33):332102.
17. Ginoza M, Yasutomi M (1999) Measurable Structure Factor of a Multi-Species Polydisperse Percus-Yevick Fluid with Schulz Distributed Diameters. *Journal of the Physical Society of Japan* 68(7):2292–2297.
18. Yang W (2003) Improved recursive algorithm for light scattering by a multilayered sphere. *Applied Optics* 42(9):1710.
19. Kim SH, et al. (2019) Solution-Processable Photonic Inks of Mie-Resonant Hollow Carbon-Silica Nanospheres. *Small* p. 1900931.

20. van Ginneken B, Stavridi M, Koenderink JJ (1998) Diffuse and Specular Reflectance from Rough Surfaces. *Applied Optics* 37(1):130.
